# Supplementary material for: Sub micron-precision sample holder for accurate re-positioning of samples in Scanning Force Microscopy
Source: arXiv:1211.2275 ancillary file (2012-11-10)
Supplement: Supplementary file 1 [file AdditionalInformation.pdf]

# Additional Information for the article "Sub micron–precision sample holder for accurate re–positioning of samples in Scanning Force Microscopy"

José Abad,[1,*] Juan Francisco González Martínez,[2,†] and Jaime Colchero Paetz[2,‡]

[1] *Dep. de Física Aplicada, Universidad Politécnica de Cartagena, E-30202, Cartagena (Spain)*
[2] *Instituto Universitario de Investigación en Óptica y Nanofísica (IUOyN), Campus de Espinardo, Universidad de Murcia, E-30100 Murcia (Spain)*

(Dated: November 9, 2012)

Scanning Probe Microscopy allows for extreme resolution down to the atomic scale. Unfortunately, total scanning range is rather limited, therefore finding a specific position on the sample is tedious. This is an important limitation of many Scanning Probe Microscopes, in particular when the sample has to be removed for some kind of treatment and then re–allocated to characterize the same position where the previous experiment had been performed. In the present work we describe two simple and compact sub micron–precision sample holders that can be easily integrated in to a commercial Scanning Force Microscopy system. The design is based either on a traditional kinematic mounting or on self–adjustment of the sample holder and the upper piece of the piezoelectric scanner as the glue used to assemble the final setup solidifies. With these sample holders a specific sample position is automatically recovered to within about 100 nanometers, and thus well within the typical range of a piezoelectric scanner. Our experimental setup therefore allows ex–situ manipulation of the sample and SFM imaging of the same region without the aid of an optical microscope, positioning marks and tedious re–allocation.

PACS numbers: 07.79.Lh
Keywords: Scanning Force Microscopy, Kelvin coupling, kinematic mount, non–kinematic mount.

* jabad@um.es
† jfgm@um.es
‡ colchero@um.es

## I. ADDITIONAL INFORMATION

As discussed in the main text, a statistically significant amount of data has to be acquired for each type of experiment in order to estimate the performance of the different sample holders, as well as of individual positioning and re–positioning actions (coarse tip sample approach and head removal). These data have to be processed in an appropriate way in order to extract the re–positioning accuracy of the different actions. In the present *additional information*, a precise description of the procedures that have been used as well as of the acquired data and the corresponding results is given. As discussed in the main text, for each type of allocation and re–allocation experiment, a series of SFM images is acquired. In addition to the topography, also amplitude –which is the channel used for the feedback– and frequency shift images are acquired. Moreover, for each channel images corresponding to forward and backward scan are saved. These SFM images were processed as follows: first, all images of the same data type (topography forward, topography backward, amplitude forward, . . .) are combined to obtain a "movie". For this combination the free WSxM software can be used. In addition, the WSxM software has a routine for "movie drift correction" that automatically computes the cross-correlation between images and finds the position of the maximum of the cross–correlation, which directly corresponds to the offset between images of the movie. We have used the option "correlate with first frame", which in our case resulted in the best "drift correction". This routine of the WSxM software determines not only the "drift–corrected movie" but also a path with the offset vectors corresponding to the calculated distance between successive images. In our experiments, these offset vectors correspond to the repositioning errors between successive removal and realignment cycles. Combining these offset vectors, a path is obtained that shows the relative tip–sample movement after each re–allocation experiment. Figure 1 shows such a "movie" together with the path calculated from *topography forward* images for a type I experiment were tip was retracted from and then approached to the sample using the micrometer screw of the SFM system (see main text).

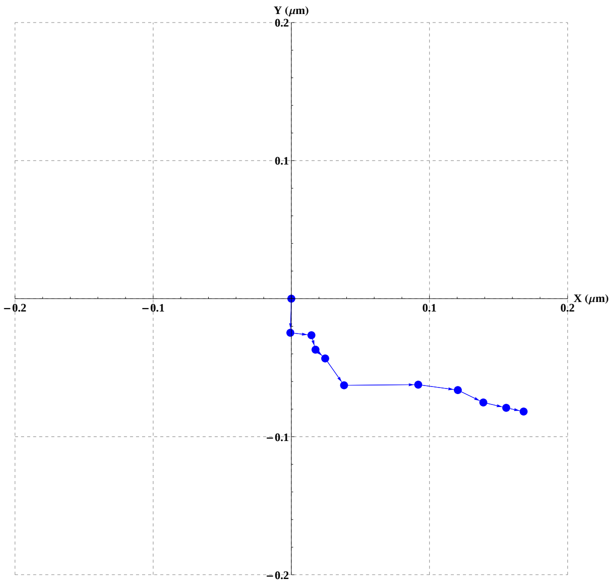


Figure 1. data (shown as "movie", left side) and path of the relative tip-sample position for a type I experiment (right side).

Since different kinds of images are acquired for each allocation and re-allocation experiment, several of these "drift-corrected movies" can be computed as well as the corresponding paths. We have used "drift-corrected movies" corresponding to *topography forward, topography backward, amplitude forward* and *amplitude backward* images. Therefore, in total 4 "movies" are obtained for the same allocation and re-allocation experiment, resulting in redundant data that can be used to estimate the accuracy of the data processing. We note that if data acquisition and processing were ideal, exactly the same paths should be obtained from each "drift–corrected movie" of the same experiment, since the corresponding frames of the 4 movies (of the same experiment) correspond to images obtained simultaneously at the same (real) tip–sample position. From the four different positions calculated from the "movies" a mean position and a statistical error can be obtained. Figure 2 shows the curves obtained from *topography images* (forward and backward), from *amplitude images* (forward and backward) and from all four curves for images corresponding a type I experiment (same experiment as discussed in figure 1). The statistical errors are shown as ellipses around the mean data points.

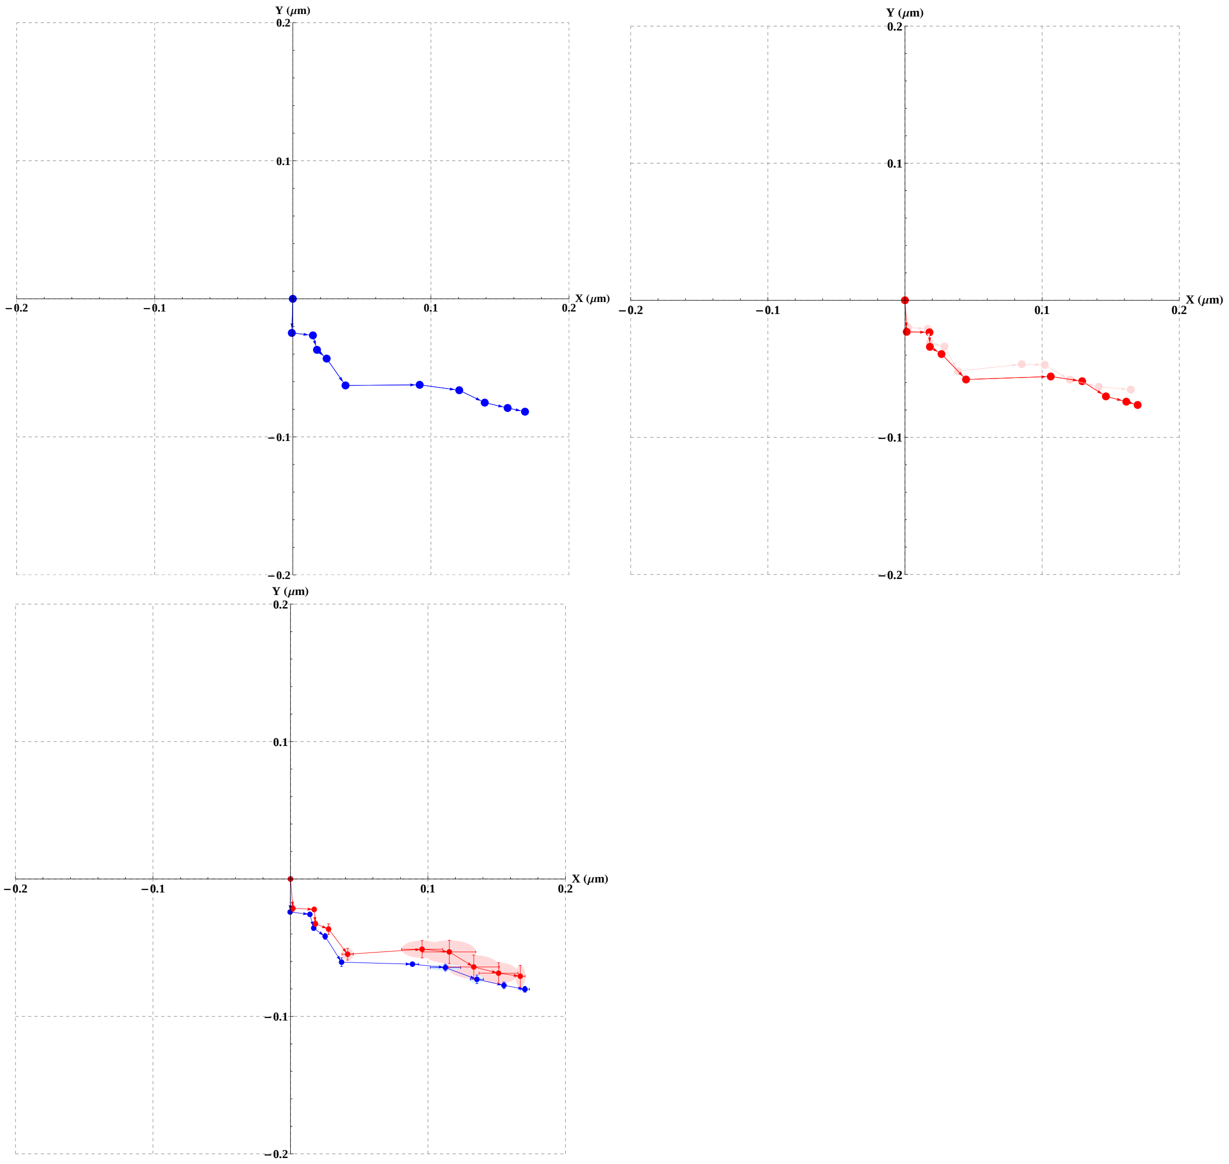


Figure 2. Processed curves for a type I experiment. First row: drift path topo (left) and drift path amplitude (right). Second row: drift path all + error (left) and drift path movie (right).

Below, the data corresponding to the experiments of type II (figure 3), $\mathrm{III}_{KC}$ (figure 4) and $\mathrm{III}_{NK}$ (figure 5) are shown. The raw data for all experiments are listed in Table I.

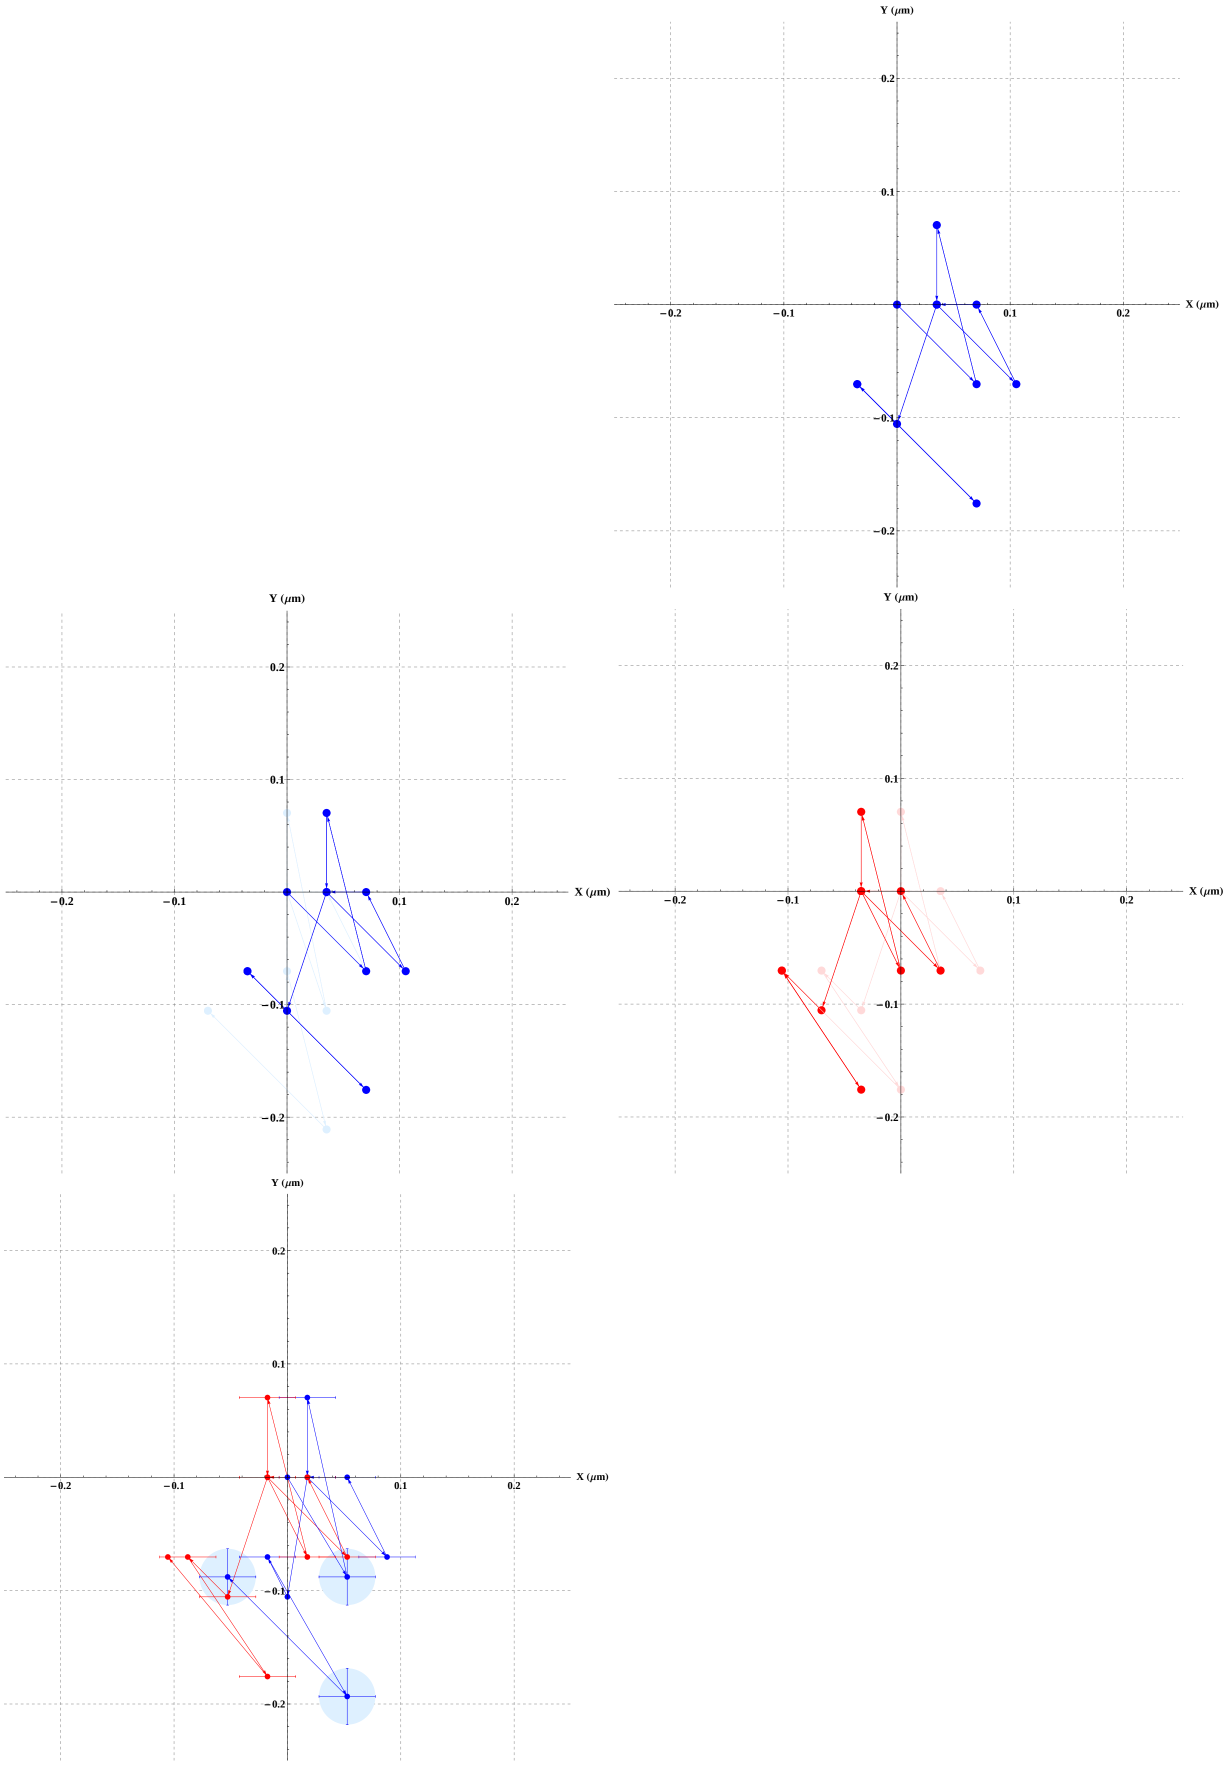


Figure 3. Data and processed curves for a type II experiment. First row: movie from topo (right) and its error path topo. Second row: drift path topo (left) and drift path amplitude (right). Third row: drift path all + error (left) and drift path movie (right).

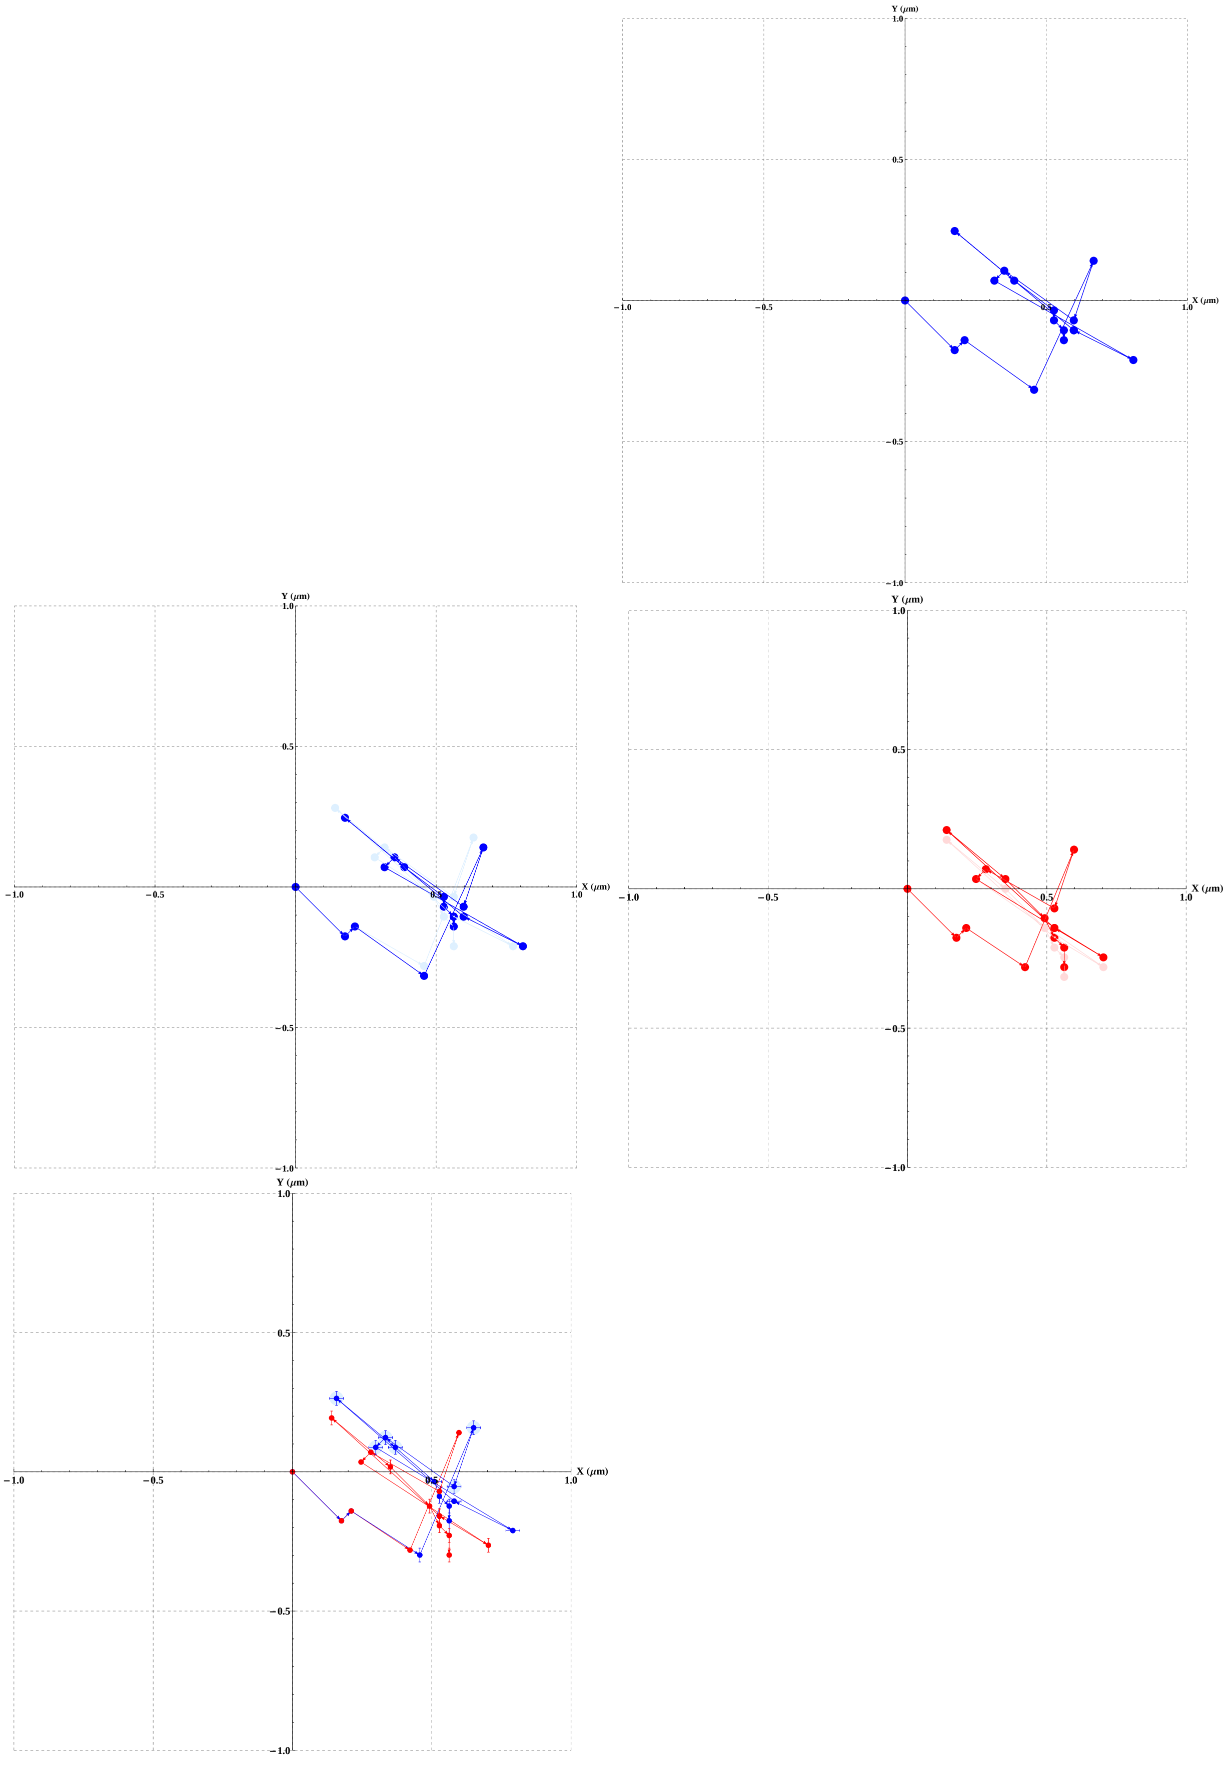


Figure 4. Data and processed curves for a type $\mathrm{III}_{KC}$ experiment. First row: movie from topo (right) and its error path topo. Second row: drift path topo (left) and drift path amplitude (right). Third row: drift path all + error (left) and drift path movie (right).

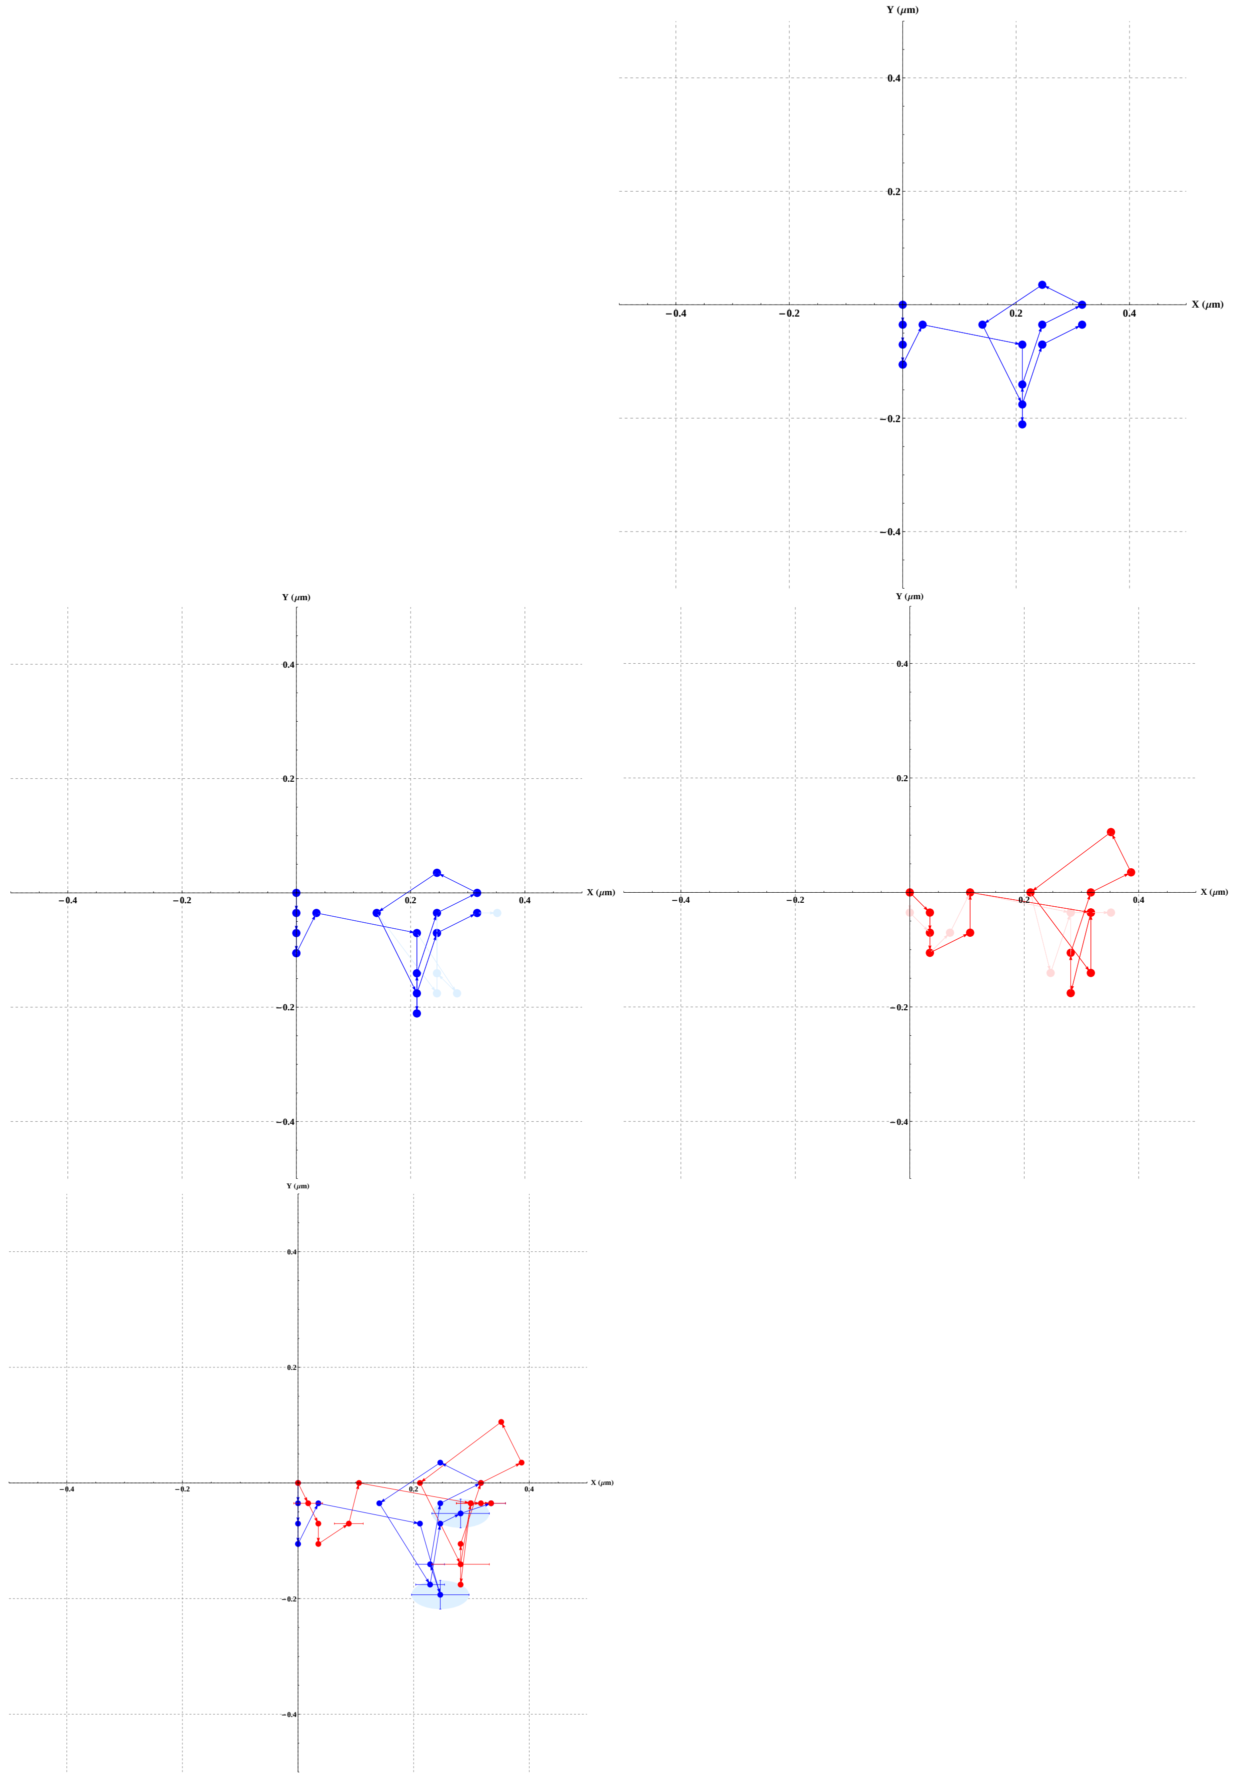


Figure 5. Data and processed curves for a type $III_{NK}$ experiment. First row: movie from topo (right) and its error path topo. Second row: drift path topo (left) and drift path amplitude (right). Third row: drift path all + error (left) and drift path movie (right).

| I (nm) | | II (nm) | | $III_{NK}$(nm) | | $III_{KC}$(nm) | |
|---|---|---|---|---|---|---|---|
| $r_i$ | $r_i - r_j$ | $r_i$ | $r_i - r_j$ | $r_i$ | $r_{i-}r_j$ | $r_i$ | $r_i - r_j$ |
| (0,0) | - | (0,0) | - | (0,0) | - | (0,0) | - |
| (1,-22) | (-1,22) | (44,-79) | (-44,79) | (9,-35) | (-9,35) | (175,-176) | (142,230) |
| (15,-24) | (-14,1) | (9,70) | (35,-149) | (18,-70) | (-9,35) | (211,-141) | (28,29) |
| (17,-34) | (-2,10) | (9,0) | (0,70) | (18,-105) | (0,35) | (439,-281) | (136,233) |
| (27,-38) | (-10,5) | (79,-70) | (-70,70) | (44,-88) | (-26,-18) | (615,158) | (307,237) |
| (39,-57) | (-12,18) | (44,0) | (35,-70) | (70,-18) | (-26,-70) | (545,-53) | (184,219) |
| (91,-56) | (-52,0) | (9,0) | (35,0) | (255,-53) | (-185,35) | (299,105) | (279,173) |
| (110,-58) | (-20,2) | (-18,-105) | (26,105) | (264,-185) | (-9,132) | (264,70) | (46,46) |
| (133,-67) | (-23,10) | (-44,-70) | (26,-35) | (255,-123) | (9,-62) | (738,-237) | (296,499) |
| (153,-72) | (-20,5) | (26,-185) | (-70,114) | (281,-18) | (-26,-105) | (545,-132) | (214,135) |
| (170,-75) | (-17,3) | (-70,-79) | (97,-105) | (352,18) | (-70,-35) | (545,-132) | (0,0) |
| - | - | - | - | (299,70) | (53,-53) | (141,237) | (510,308) |
| - | - | - | - | (176,-18) | (123,88) | (352,62) | (153,250) |
| - | - | - | - | (255,-158) | (-79,141) | (492,-79) | (114,184) |
| - | - | - | - | (272,-53) | (-18,-105) | (527,-149) | (50,77) |
| - | - | - | - | (299,-44) | (-26,-9) | (563,-185) | (28,77) |
| - | - | - | - | (334,-35) | (-35,-9) | (563,-255) | (53,46) |

Table I. Raw data points of the paths obtained for the different re–allocation experiments (I, II, $III_{KC}$ and $III_{NK}$).
